# Supplementary material for: A Neural-enhanced Factor Graph-based Algorithm for Robust Positioning in Obstructed LOS Situations
Source: arXiv:2308.15972 source file (2023-11-29)
Supplement: Supplementary file 1 [file appendix.tex]

\section{Derivation of the data association prior}

lalalalal
